# Supplementary material for: DinoLizer: Separating VAE and Diffusion Artifacts in Generative Inpainting Localization
Source: arXiv:2511.20722 source file (2026-07-30)
Supplement: Supplementary file 1 [file supplement_materials.pdf]

# DinoLizer:

## Learning from the Best for Generative Inpainting Localization

### Supplementary Material

#### A. Implementation Details

As outlined in Section 5.3, DinoLizer is based on a ViT-B/14 backbone with registers, refined on the B-Free dataset [13]. To train its linear classification head we adopted the following hyper-parameter configuration:

- batch size: 64,
- initial learning rate:  $10^{-3}$ ,
- learning rate scheduler: `lrdrop` decreasing the learning rate by half whenever the validation loss does not improve for four consecutive epochs,
- optimizer: `adamW`,
- weight decay:  $10^{-5}$ .

The training was capped at 100 epochs, with early stopping triggered once the learning rate fell below  $10^{-6}$ . The best validation performance was achieved after 15 epochs with each epoch lasting 42 minutes on a single NVIDIA V100 GPU with 32GB of memory.

#### Augmentations

To robustify the detector against common image processing operations, while still training on images of size  $H \times W = 504 \times 504$ , we used the following combination of augmentations implemented with the Albumentations library (<https://albumentations.ai/>):

- Random horizontal flip with probability 0.5 ( $p = 0.5$ ),
- Random rotation by  $90^\circ$  ( $p = 1$ ),
- One of the following, each with  $p = 0.25$ :
  1. `RandomResizedCrop` to size  $H \times W$  with scale factor uniformly sampled from  $(0.1, 1)$  and aspect ratio fixed at 1,
  2. `RandomCrop` to size  $H \times W$ ,
  3. Resizing directly to size  $H \times W$ ,
  4. Upscaling by either 200% or 300%, followed by `RandomCrop` to size  $H \times W$ ,
- Uniform box blur with kernel size  $k \in \{3, 4, 5\}$  ( $p = 0.1$ ),
- Gaussian noise with standard deviation  $\sigma$  uniformly sampled from  $(0.2, 0.44)$  ( $p = 0.1$ ),
- Color jitter ( $p = 0.1$ ),
- First JPEG compression with quality factor  $QF$  uniformly drawn from  $\{40, \dots, 100\}$  ( $p = 0.5$ ),
- Optional second JPEG compression with quality factor  $QF_2$  drawn from  $\{40, \dots, 100\}$  ( $p = 0.1$  if first compression applied).

All resizing operations employ Lanczos interpolation.

| Dataset          | min-max<br>H | min-max<br>W | mask size<br>$\bar{m}$ | $\bar{m}_W$ |
|------------------|--------------|--------------|------------------------|-------------|
| BtB [1]          | 234 – 1152   | 246 – 1152   | 0.22                   | 0.27        |
| B-Free [13]      | 512          | 512          | 0.47                   | 0.59        |
| COCO [12]        | 256          | 256          | 0.25                   | 0.32        |
| TGIF [24]        | 518 – 1024   | 539 – 1024   | 0.06                   | 0.12        |
| SAGI-<br>SP [11] | 144 – 4928   | 200 – 4928   | 0.19                   | 0.31        |
| FR [11]          | 139 – 2048   | 216 – 2048   | 0.20                   | 0.27        |

Table 5. Overview of evaluation datasets with their image sizes ( $H$  - height range,  $W$  - width range), their average relative mask size  $\bar{m}$ , and average mask size  $\bar{m}_W$  per overlapping (modified) windows of size  $504 \times 504$  with stride  $S = 128$ .

During validation, we accelerate the evaluation by applying only a center crop followed by JPEG compression with a randomly selected quality factor between 40 and 100, applied with probability  $p = 0.5$ .

#### B. Qualitative Study

To assess the robustness of our method, we evaluated its performance on several out-of-distribution datasets that were not included in the training set, as described in Section 4.1. These datasets differ both in their image sources and the generative models employed (see Table 1) and exhibit a wide range of image dimensions (Table 5). In the following analysis, we focus on two datasets, TGIF and SAGI-FR, in which DinoLizer’s performance appears suboptimal.

#### Failure case of TGIF

To understand why DinoLizer exhibits inferior performance on the TGIF dataset relative to TruFor, we analyzed the distribution of modification sizes within images. For each image (after a possible upsampling required for small inputs, as described in Section 3.3), we computed the mean mask size over overlapping sliding windows of  $504 \times 504$  pixels with stride  $S = 128$ , restricting the analysis to windows that contain at least one modified pixel. This metric reflects the typical size of alterations that DinoLizer is expected to detect within each image. We denote the mean mask size for the  $i$ -th image as  $m_W^{(i)}$ , and its average over a dataset as  $\bar{m}_W$ , which is reported in the last column of Table 5.

In the B-Free dataset (used for training) we observe that, on average, 59% of the pixels in each modified window are altered. The discrepancy with the overall average mask size  $\bar{m}$  of 47% arises because  $\bar{m}$  is computed over the images without upsampling small images and includes both mod-

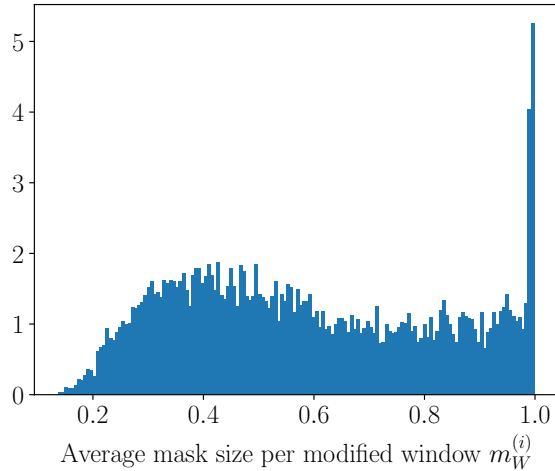

Figure 6. Histogram of average changes per modified overlapping windows of size  $504 \times 504$  with stride 128 ( $m_W^{(i)}$ ) in B-Free dataset.

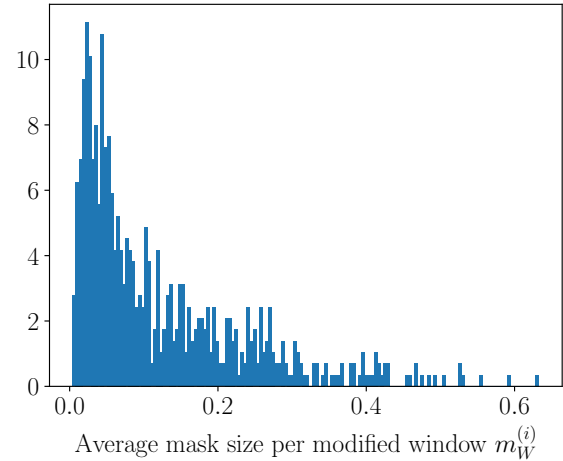

Figure 7. Histogram of average changes per modified overlapping windows of size  $504 \times 504$  with stride 128 ( $m_W^{(i)}$ ) in TGIF dataset.

ified and unmodified regions, whereas  $\bar{m}_W$  focuses exclusively on windows containing modifications.

Table 5 also shows that  $\bar{m}_W$  for TGIF is only 12%. Figure 6 demonstrates that nearly all B-Free images have  $m_W^{(i)}$  exceeding 12%, whereas Figure 7 indicates that most TGIF images exhibit  $m_W^{(i)}$  below 12%. Consequently, DinoLizer is ill-suited for detecting manipulations that occupy relatively small portions of an image (roughly 20% of a  $504 \times 504$  window, corresponding to  $225 \times 225$  pixels or smaller). This limitation is further illustrated by the last visual example in Figure 13, where a small modified region is missed. Note that the images in the visual example are scaled for better visualization and the last example is indeed smaller than the others. A straightforward remedy could be to augment the training set with small manipulated regions, but we were unable to implement this improvement in the current manuscript due to time constraints.

### Failure case of SAGI-FR

As we see in Table 2, DinoLizer’s performance decreases markedly when evaluated on the SAGI-FR dataset relative to SAGI-SP. The model is trained to classify content reconstructed by a VAE (without inpainting) as authentic, and we hypothesize that this training regime explains the observed drop. According to Table 1, the inpainting procedure employed in SAGI-FR relies on different generative models than Stable Diffusion 2 used in the B-Free dataset. Consequently, DinoLizer tends to interpret the reconstructed background in SAGI-FR images as inpainted artefacts. This behavior is corroborated by Figure 10, where DinoLizer (along with several other detectors) achieves higher F1 scores as the strength of post-processing increases and high-

frequency traces introduced by the VAE are progressively attenuated. Further visual evidence is presented in Figure 14.

## C. Additional Robustness Results

To provide a comprehensive assessment of the robustness of our proposed localizer, we present F1-score curves for the four missing benchmark datasets missing in the main part of the paper: Beyond the Brush (Figure 8), TGIF (Figure 9), SAGI-FR (Figure 10), and B-Free (Figure 11). Across these datasets, the trends mirror those observed for CocoGlide and SAGI-SP in Section 4.2: DinoLizer maintains a relatively stable performance across varying degrees of post-processing, consistently achieving higher F1 scores than competing detectors.

The only notable deviations appear on TGIF, where TruFor outperforms DinoLizer on unprocessed images, and on SAGI-FR, where DinoLizer (along with other detectors) benefits from more aggressive post-processing. These deviations are consistent with the explanations provided in the preceding section.

## D. Additional Visual Results

For completeness, we provide visual examples of predictions on additional datasets: Beyond the Brush (Figure 12), TGIF (Figure 13), SAGI-FR (Figure 14), SAGI-SP (Figure 15), and B-Free (Figure 16).

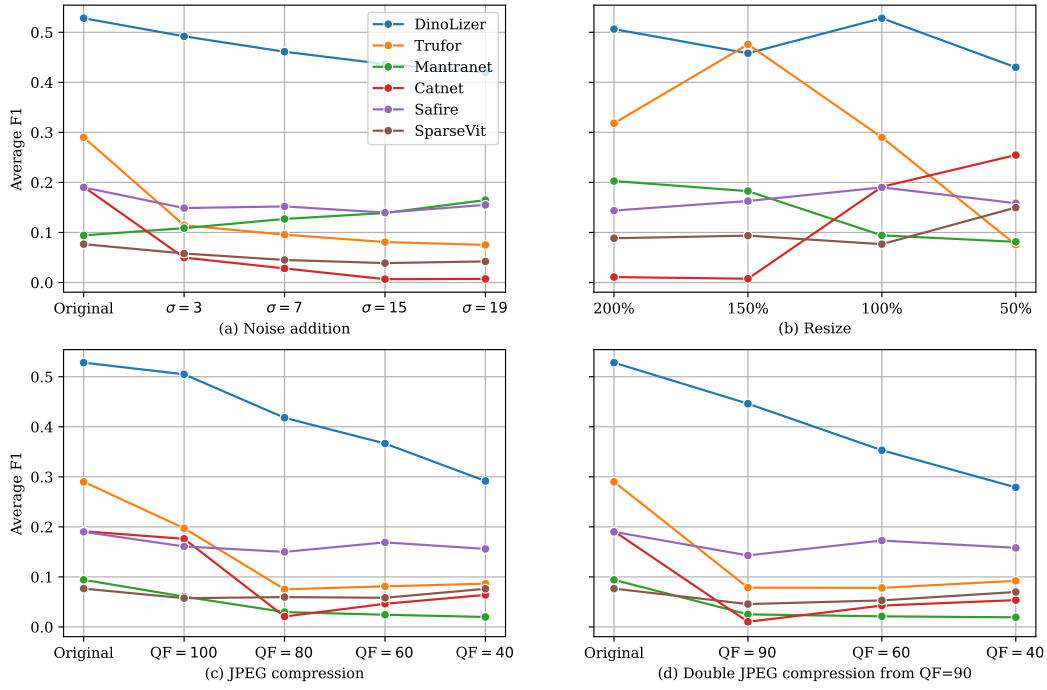

Figure 8. F1 score performance under different types of perturbations on Beyond the Brush: (a) gaussian noise, (b) resizing, (c) JPEG compression, and (d) double JPEG compression.

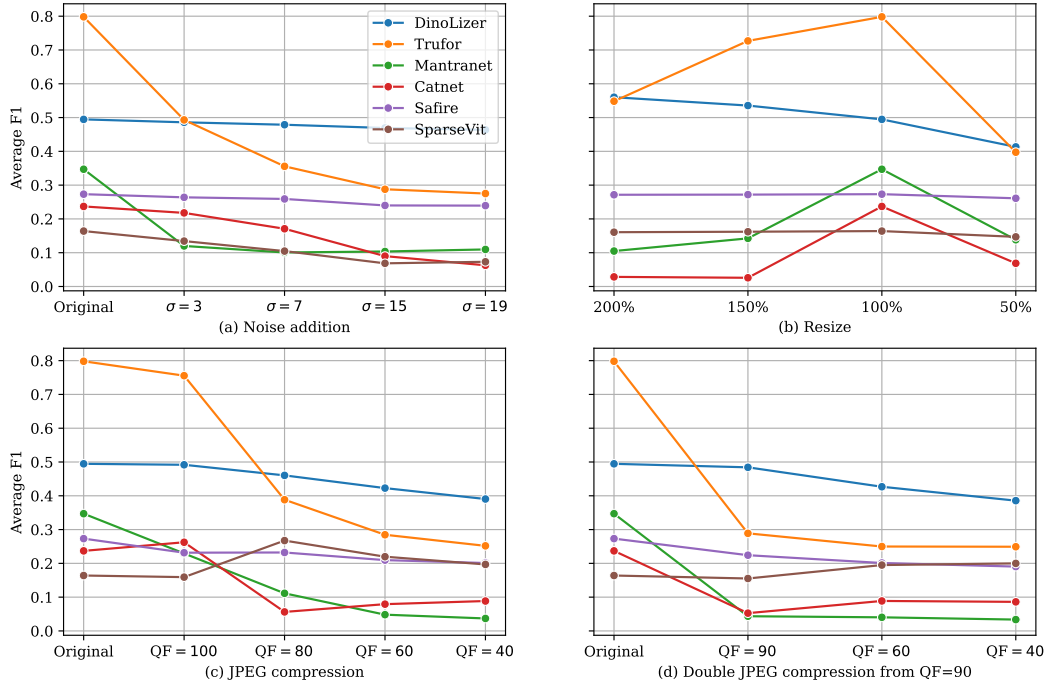

Figure 9. F1 score performance under different types of perturbations on TGIF: (a) gaussian noise, (b) resizing, (c) JPEG compression, and (d) double JPEG compression.

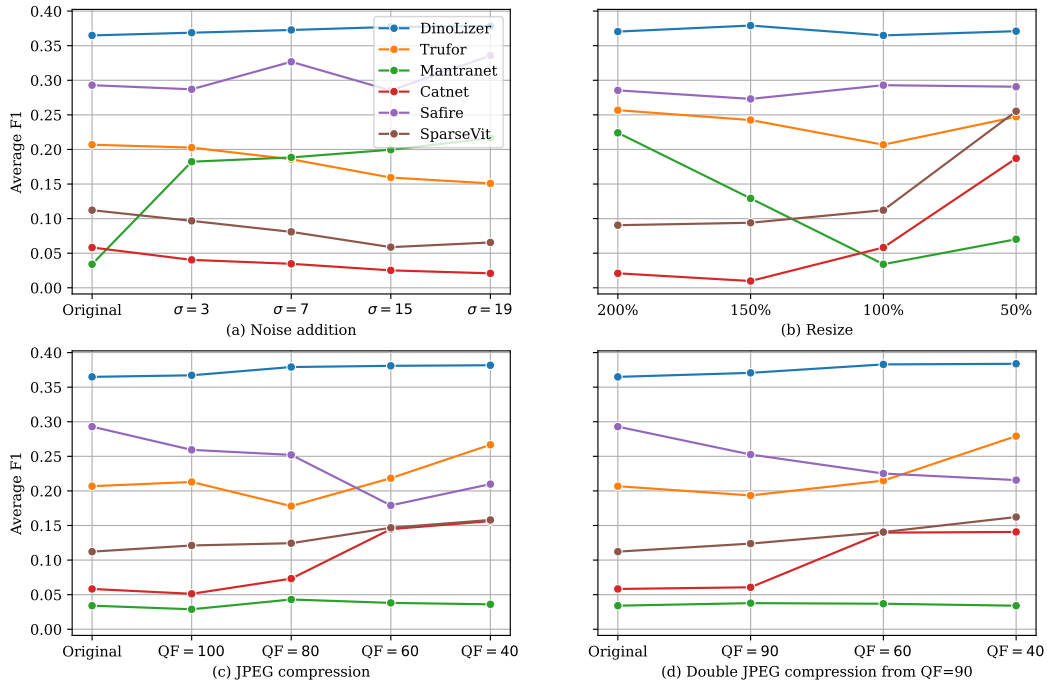

Figure 10. F1 score performance under different types of perturbations on SAGI-FR: (a) gaussian noise, (b) resizing, (c) JPEG compression, and (d) double JPEG compression.

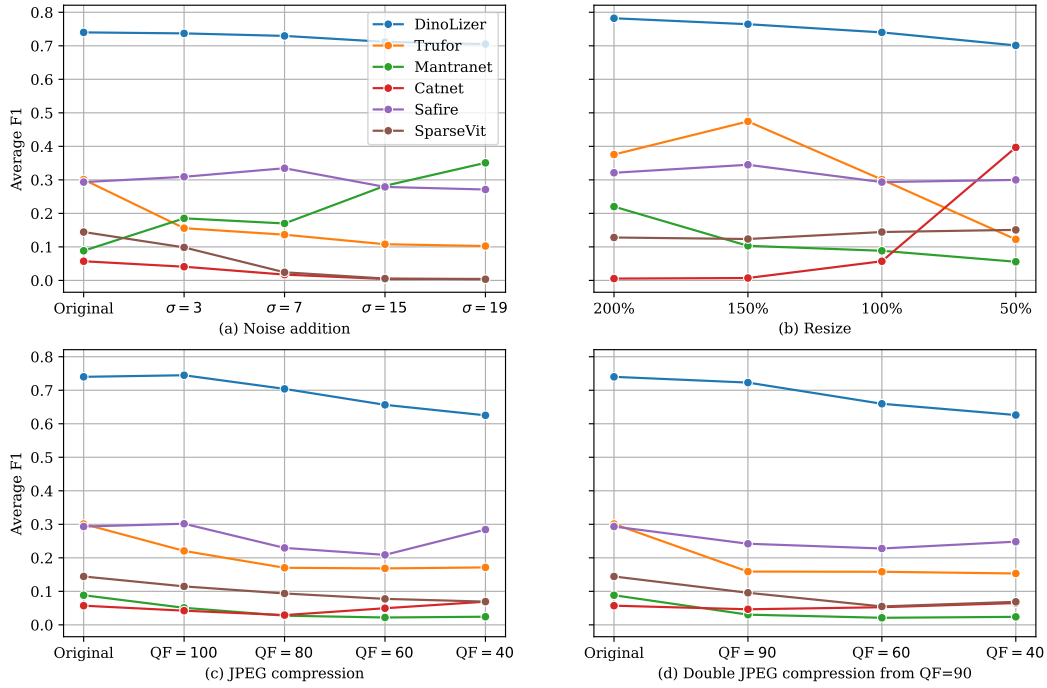

Figure 11. F1 score performance under different types of perturbations on B-Free: (a) gaussian noise, (b) resizing, (c) JPEG compression, and (d) double JPEG compression.

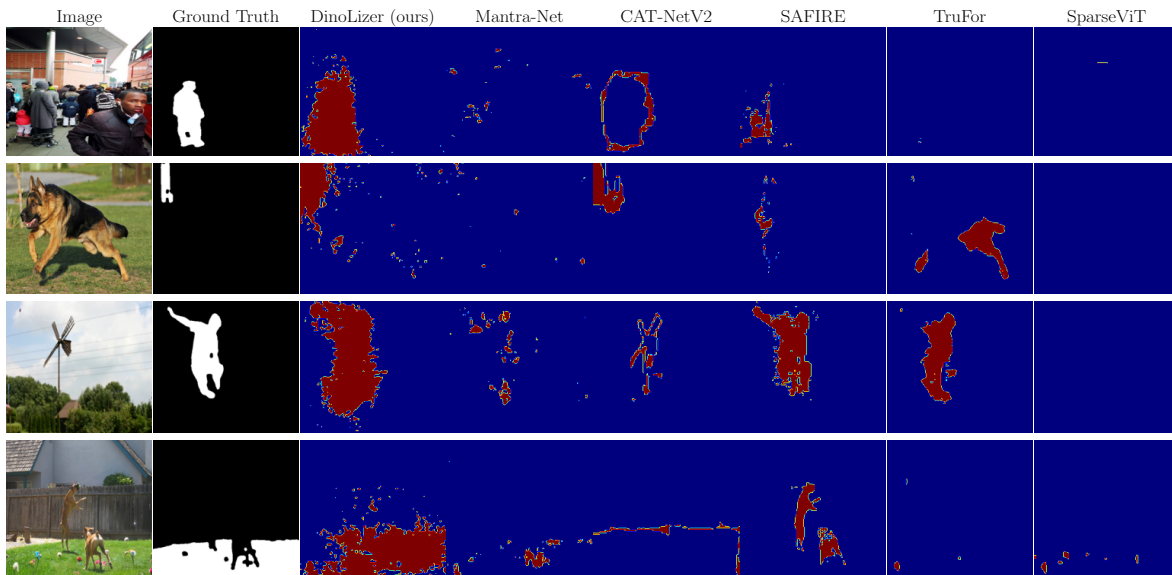

Figure 12. Visual comparison of forgery localization results on the Beyond the Brush dataset.

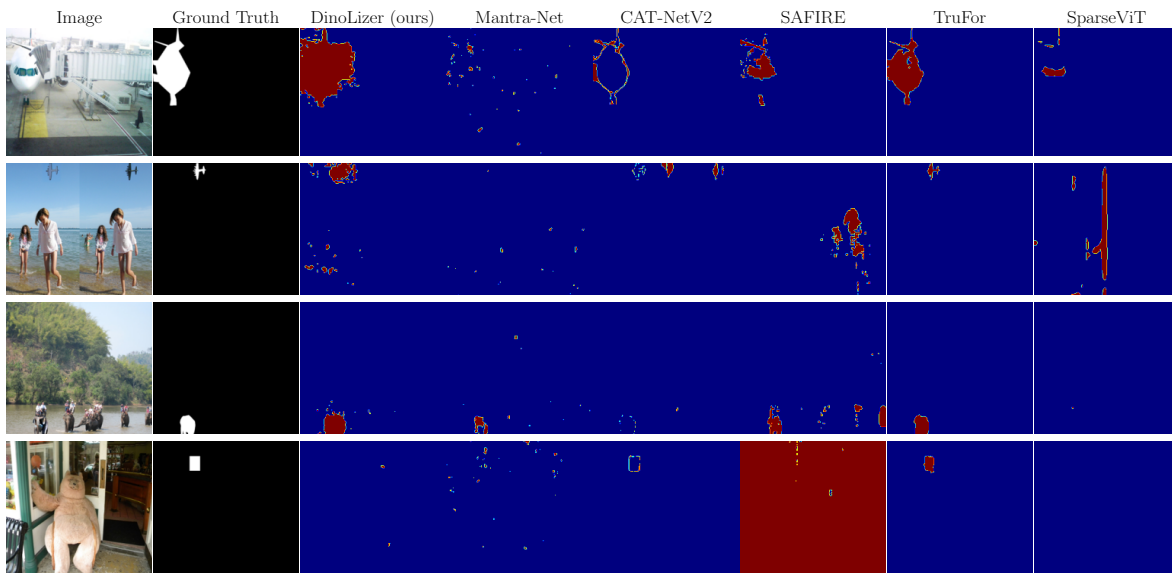

Figure 13. Visual comparison of forgery localization results on the TGIF dataset.

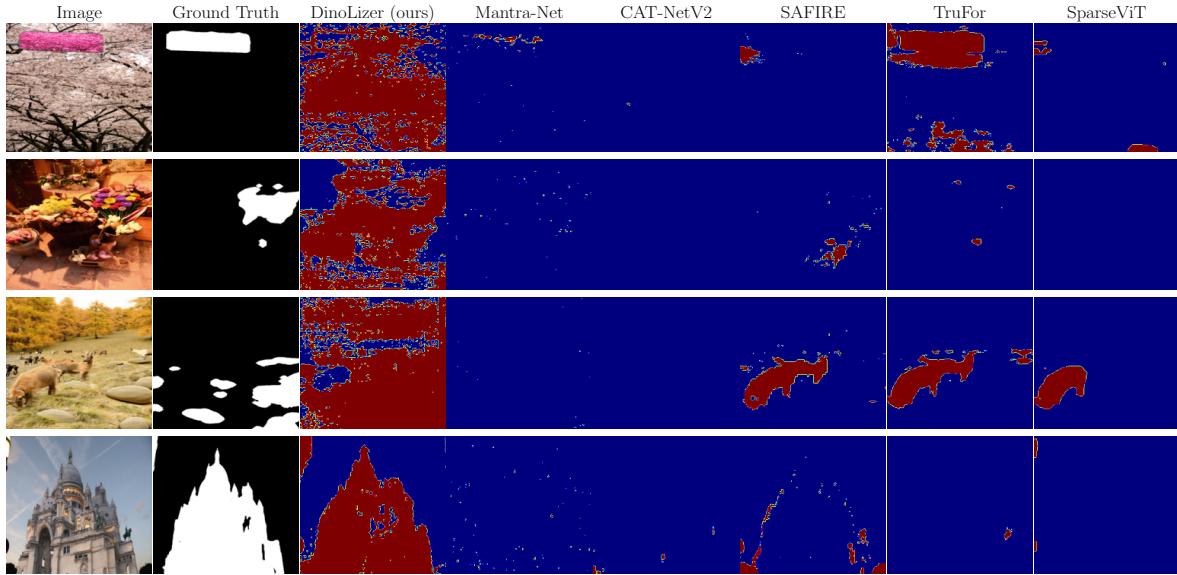

Figure 14. Visual comparison of forgery localization results on the SAGI-FR dataset.

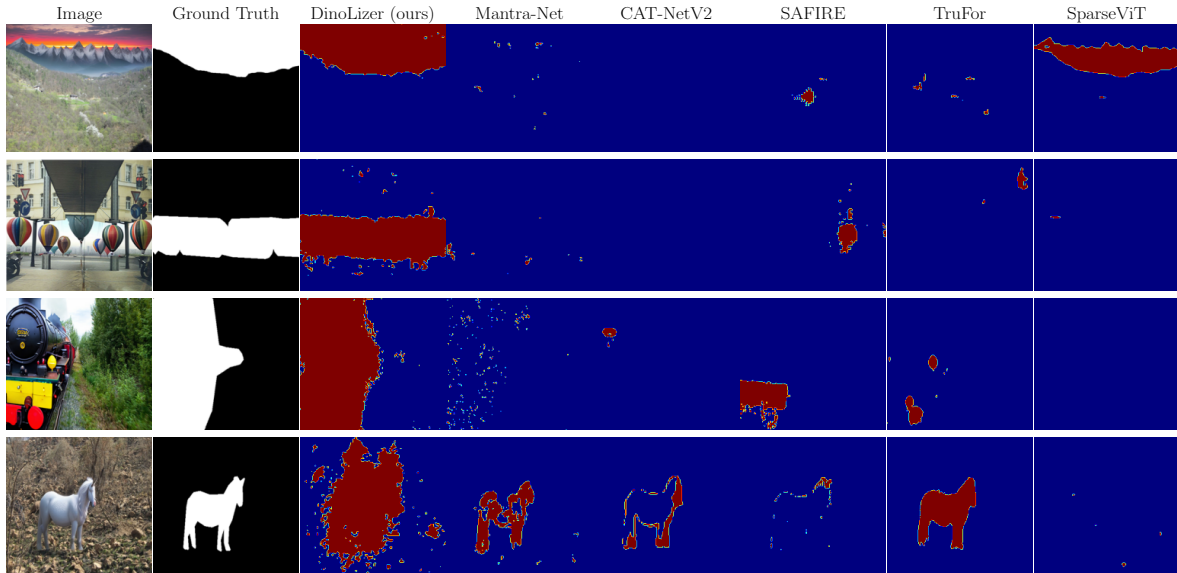

Figure 15. Visual comparison of forgery localization results on the SAGI-SP dataset.

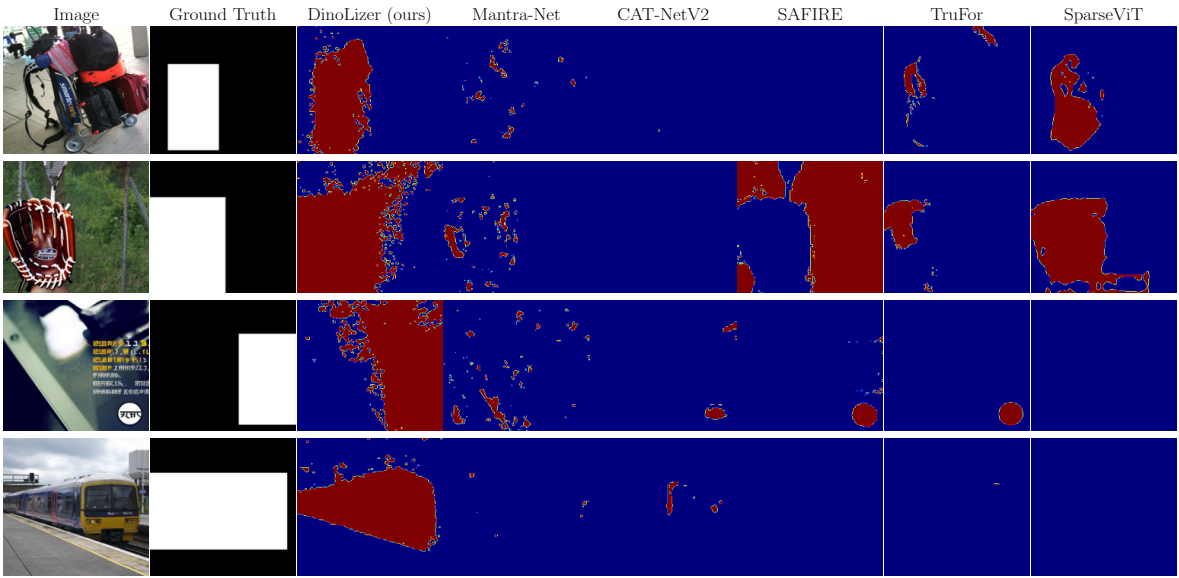

Figure 16. Visual comparison of forgery localization results on the B-Free dataset.
